# Supplementary material for: Effective and General Distance Computation for Approximate Nearest Neighbor Search
Source: arXiv:2404.16322 source file (2025-01-17)
Supplement: Supplementary file 1 [file appendix.tex]

\clearpage
\section*{Appendix}
%\nobalance

\subsection{The Proofs}

\stitle{Proof of Lemma~\ref{lem:var=quantile}.}
We get $\epsilon\sim\mathcal{N}(0, \sigma^2)$ under the Gaussian distribution assumption. The error quantile can be expressed by the inverse CDF (quantile function) of the Gaussian distribution with probability $q$:
\begin{equation*}
F^{-1}(p)=\mu + \sigma\sqrt{2} \mathrm{erf}^{-1} (2p-1)
\end{equation*}
The $\mathrm{erf}^{-1}(x)$ is the inverse function of the error function and is positive for $x>0$.
When the probability $p$ is fixed, $\mu=0$ by centralized, only $\sigma$ affects the value.  Then the variance of the error is minimized, and the right quantile($p>0.5$) of the error is also minimized

\stitle{Proof of Theorem~\ref{theorem:PCA}.}
First, we consider the simplest case where the projection dimension $d=1$. 
We define a vector $\ww_1 \in \mathbb{R}^D$ as the direction of the lower dimensional space. As we are only interested in the direction of the space, we set $\ww_1$ to be of unit length where $\ww_1^T\ww_1=1$. Then the vector $\xx_n$ can be projected onto this new space as $\hat{\xx}_n=\ww_1^T\xx_n$. 
We define $ \bar \xx$ as the mean of the $\xx \in S$ in the original space, and the mean of the vectors in the projected space is given by $ \hat{\bar \xx}= \ww_1^T\bar \xx$. 
We can write the variance of the projected data as:
    \begin{equation*}
        \begin{aligned}
        \sigma^2(\hat{\xx})& =\frac1N\sum_{n=1}^N(\hat{\xx}_n-\hat{\bar{\xx}})^2  \\
        &=\frac1N\sum_{n=1}^N(\ww_1^T\xx_n-\ww_1^T\bar{\xx})^2 \\
        % &=\frac1N\sum_{n=1}^N(\ww_1^T\xx_n-\ww_1^T\bar{\xx})(\ww_1^T\xx_n-\ww_1^T\bar{\xx})^T \\
        % &=\frac1N\sum_{n=1}^N(\ww_1^T\xx_n-\ww_1^T\bar{\xx})(\xx_n^T\ww_1-\bar{x}^T\ww_1) \\
        % &=\frac1N\sum_{n=1}^N\ww_1^T(\xx_n-\bar{\xx})(\xx_n^T-\bar{\xx}^T)\ww_1 \\
        &=\frac1N\sum_{n=1}^N\ww_1^T(\xx_n-\bar{\xx})(\xx_n-\bar{\xx})^T\ww_1 \\
        &=\ww_1^T\Sigma \ww_1
        \end{aligned}
    \end{equation*}
    where $\Sigma$ is the covariance matrix. To minimize the residual dimension variance, we consider the stationary point of the above equation. Whether maximizing or minimizing the above formulas, we introduce a Lagrange multiplier $\lambda_1$ and formulate our optimization objective as follows:
    \begin{equation*}
        J(\ww_1)=\ww_1^T\Sigma \ww_1 + \lambda_1(1-\ww_1^T\ww_1)
    \end{equation*}
    with the unit norm constraint $\ww_1^T\ww_1=1$. Setting the derivative of the above equation, we get a stationary point when,
    \begin{equation*}
    \begin{aligned}
                \frac{\partial J(\ww_{1})}{\partial \ww_1}=2&\Sigma \ww_{1}-2\lambda_{1}\ww_{1}=0 \\
                % &\Sigma w_1=\lambda_1 w_1 \\
                % w_1^T &\Sigma w_1=\lambda_1 w_1^Tw_1 \\
                \ww_1^T &\Sigma \ww_1=\lambda_1
    \end{aligned}
    \end{equation*}
    This shows that at the stationary point, $\ww_1$ must be an eigenvector of $\Sigma$ and $\lambda_1$ the eigenvalue. we can see that the maximum or minimum variance is equal to the eigenvalue $\lambda_1$. We can identify additional principal components by choosing directions that maximize variance while being orthogonal to the existing ones. For the general case of a lower dimensional space with $d$ dimensions with $d<D$, the principal components are the eigenvectors $\ww_1, \ww_2 ... \ww_d$ corresponding to the $d$ largest eigenvalues $\lambda_1, \lambda_2 ... \lambda_d$ and the residual dimension corresponding the $r$ smallest eigenvalues $\lambda_{d+1}, \lambda_{d+2} ... \lambda_{r}$. Then we can prove the PCA matrix $[\ww_1 ... \ww_D]^T$ maximizes the projection dimension variance which also minimizes the residual dimension variance.

\input{figures/result_plot_ip}
%\vspace{-1em}

\input{figures/result_plot_ood}

\vspace{-2em}

\input{figures/result_plot_retrain}

\input{figures/result_plot_avx}

\subsection{Additional Experiments}
We first present more implementation details, followed by a presentation of additional experimental results.

\stitle{More Implementation Details.}
For the random projection approach, we set $\epsilon_0=2.1$ and $\Delta_d=32$, following the recommendations for $\ADS$. 
For both \BSAR and \BSAP, each $\Delta_d$ was also set to 32 to maintain the same setting as $\ADS$. 
In the \BSAO approach, the subspace number was set to $d/8$ for the GIST dataset and $d/4$ for the others, since each dataset dimension is divisible by 4. 
The parameter $nbits$ for \BSAO was set to 8 as per the default. 
The target recall for both \BSAP and \BSAO methods was configured to 0.995.
For the multiplier $m$ in \BSAR, values were set to 8 for the SIFT, GIST, and DEEP datasets, 12 for TINY and WORD2VEC, and 16 for the GlOVE dataset. 
In cases involving adaptive adjustment of classifiers, the target recall for each classifier was determined based on $\Delta_d$, calculated as $r_i = \left(1 - \frac{1 - r}{D/\Delta_d}\right)$.
Upon receiving a query, the algorithm first applies a transformation through matrix multiplication, implemented with the C++ Eigen library. 
%This operation takes approximately 0.344 ms on the GIST dataset.
%Specifically, the projection time represents only 6\% of the total time cost when achieving a recall rate above 90\%, and reduces further to just 3\% at a 95\% recall rate. 
%Moreover, the time complexity for computing the lookup table constitutes only 1\% to 2\% of the overall computation time.

\begin{revise}
\stitle{Exp-A.1. Test of Inner Product.}
Note that our \BSAR method can be easily adapted for maximum inner product search by omitting the norm term in the distance estimation. 
In this case, the (exact) inner product can be decomposed as follows:
\begin{equation}
\begin{aligned}
    \Braket{\qq, \xx} = \Braket{\qq_D, \xx_D} = \Braket{\qq_d, \xx_d} + \Braket{\qq_r, \xx_r},
\end{aligned}
\label{eq:ip-decomp}
\end{equation}
where the error term remains consistent with the original \BSAR method. 
This allows the approximate distance to be computed as $\Braket{\qq_d, \xx_d}$ in $O(d)$ operations.

We continue to apply PCA projection to minimize the variance of the error term and use the Gaussian assumption to prune distance computations effectively.
The results, shown in Fig.~\ref{fig:ip-time-acc-trade}, indicate \BSAR achieves a 1.5x to 2x speedup compared to the original $\HNSW$ algorithm on DEEP.

\stitle{Exp-A.2. Effect of Out-of-Distribution Queries.}
Out-of-distribution (OOD) data poses a big challenge for data-driven learning methods. 
To assess the performance of our approach on OOD queries, we introduce Gaussian noise to the original queries and perform experimental evaluations. 
The results, presented in Fig.~\ref{fig:ood-time-acc-trade}, demonstrate that our algorithms, \BSAR and \ADS, are relatively robust against OOD queries. 
This robustness arises because \ADS operates as a data-free method, leveraging error bounds based on the Johnson-Lindenstrauss (JL) lemma derived from random matrices. 
In contrast, the \BSAR algorithm considers the query as a deterministic variable, enhancing its effectiveness for handling OOD queries. 
In comparison, the \BSAP and \BSAO algorithms exhibit limitations under OOD conditions, as they tend to suffer from either lower efficiency or reduced recall in these scenarios.

\stitle{Exp-A.3. Test of Handling Out-of-Distribution Queries.}
To address the challenge of out-of-distribution (OOD) queries, a practical approach involves retraining the linear classifier. By utilizing 100 queries and requiring approximately 10 seconds, this method enables rapid model adaptation. As demonstrated in Fig.~\ref{fig:retrain-time-acc-trade}, our experimental results indicate that this retraining strategy effectively mitigates accuracy degradation of the linear model in OOD scenarios.

\stitle{Exp-A.4: Additional Results on Comparison with FINGER.}
In Exp-4 of \S~\ref{sec:experiment}, we presented a comparison with FINGER on the GIST and DEEP datasets. 
In this section, we provide additional results on other datasets, which are displayed in Fig.~\ref{fig:avx512-time-acc-trade}. The results are consistent with those in Exp-4, so we omit further discussion for brevity.

\end{revise}
